# Supplementary material for: On the Privacy of dK-Random Graphs
Source: arXiv:1907.01695 source file (2019-07-03)
Supplement: Supplementary file 1 [file appendix.tex]

\section{Appendix}
\label{sec:appendix}

\begin{table*}
	
	\caption{Dataset: fb107, Basic graph properties of 1k graphs, overlap $\alpha=0.2$ and choice BFS-Tree (Highest Degree)}
	\label{tbl:dk_fb107}
	\begin{tabular}{|c||>{\columncolor[gray]{0.8}}c||c|c|c|c||>{\columncolor[gray]{0.8}}c||c|c|c|c|}
		\hline 
		metric & $G1$ & $G1_1$ & $G1_2$ & $G1_3$ & $G1_4$  & $G2$ & $G2_1$ & $G2_2$ & $G2_3$ & $G2_4$\\ 
		\hline \hline
		$|N|$ & 614 & 612 & 612 & 612 & 612 & 617 & 613 & 613 & 613 & 613 \\ 
		\hline 
		$|E|$ & 15554 & 15553 & 15553 & 15553 & 15553 & 13577 & 13575 & 13575 & 13575 & 13575\\ 
		\hline 
		avg-degree & 50.6645 & 50.8268 & 50.8268 & 50.8268 & 50.8268 & 44.0097 & 44.2904 & 44.2904 & 44.2904 & 44.2904 \\ 
		\hline 
		degree-assortavity 	& 0.3766 & -0.1267 & -0.1284 & -0.1208 & -0.1373 & 0.3905 & -0.1295 & -0.1284 & -0.13 & -0.1253 \\ 
		\hline 
		clustering & 0.5346 & 0.3192 & 0.3198 & 0.3219 & 0.3254 & 0.5247 & 0.3143 & 0.32 & 0.3178 & 0.3181 \\ 
		\hline 
		avg-distance & 2.833 & 2.1222 & 2.1288 & 2.1238 & 2.1184 & 3.0489 & 2.188 & 2.182 & 2.1823 & 2.1843\\ 
		\hline 
	\end{tabular} 
\end{table*}

\begin{table*}
	
	\caption{Dataset: caGrQc, Basic graph properties of 1k graphs, overlap $\alpha=0.2$ and choice BFS-Tree (Highest Degree)}
	\label{tbl:dk_caGrQc}
	\begin{tabular}{|c||>{\columncolor[gray]{0.8}}c||c|c|c|c||>{\columncolor[gray]{0.8}}c||c|c|c|c|}
		\hline 
		metric & $G1$ & $G1_1$ & $G1_2$ & $G1_3$ & $G1_4$  & $G2$ & $G2_1$ & $G2_2$ & $G2_3$ & $G2_4$\\ 
		\hline \hline
		$|N|$ & 2757 &2191&2191&2191&2191&2757&2160&2160&2160&2160 \\ 
		\hline 
		$|E|$ & 7488 &7065&7065&7065&7065&7377&6777&6777&6777&6777\\ 
		\hline 
		avg-degree & 5.43199 &6.4491&6.4491&6.4491&6.4491&5.3514&6.275&6.275&6.275&6.275 \\ 
		\hline 
		degree-assortavity 	& 0.6223 &-0.042&-0.0437&-0.0085&-0.0273&0.6268&-0.04&-0.0235&-0.0367&-0.0473 \\ 
		\hline 
		clustering & 0.4556 &0.0168&0.0228&0.0198&0.0188&0.4418&0.02&0.0187&0.02&0.02 \\ 
		\hline 
		avg-distance & 3.50417 &3.7702&3.7657&3.7556&3.778&3.3787&3.7731&3.7863&3.7878& 3.7931\\ 
		\hline 
	\end{tabular} 
\end{table*}

\begin{table*}
	
	\caption{Dataset: soc-anybeat, Basic graph properties of 1k graphs, overlap $\alpha=0.2$ and choice BFS-Tree (Highest Degree)}
	\label{tbl:dk_soc-anybeat}
	\begin{tabular}{|c||>{\columncolor[gray]{0.8}}c||c|c|c|c||>{\columncolor[gray]{0.8}}c||c|c|c|c|}
		\hline 
		metric & $G1$ & $G1_1$ & $G1_2$ & $G1_3$ & $G1_4$  & $G2$ & $G2_1$ & $G2_2$ & $G2_3$ & $G2_4$\\ 
		\hline \hline
		$|N|$ & 6666 & 6584 &6584&6584&6584&6976&6942&6942&6942&6942 \\ 
		\hline 
		$|E|$ & 22313 & 22265 &22265&22265&22265&23591&23572&23572&23572&23572\\ 
		\hline 
		avg-degree & 6.6945 & 6.7633 &6.7633&6.7633&6.7633&6.7634&6.7911&6.7911&6.7911&6.7911\\ 
		\hline 
		degree-assortavity 	& -0.13856 & -0.13816 &-0.13817&-0.13814&-0.13815&-0.1474&-0.14625&-0.1462&-0.14627&-0.1463 \\ 
		\hline 
		clustering & 0.2156  & 0.2066 &0.2051&0.2065&0.20511&0.2111&0.1994&0.2032&0.2032&0.19826 \\ 
		\hline 
		avg-distance & 2.83197 & 2.7074 &2.6905&2.72581&2.715&2.8926&2.7552&2.7428&2.7692&2.7758\\ 
		\hline 
	\end{tabular} 
\end{table*}

\begin{table*}
	
	\caption{Dataset: soc-gplus, Basic graph properties of 1k graphs, overlap $\alpha=0.2$ and choice BFS-Tree (Highest Degree)}
	\label{tbl:dk_soc-gplus}
	\begin{tabular}{|c||>{\columncolor[gray]{0.8}}c||c|c|c|c||>{\columncolor[gray]{0.8}}c||c|c|c|c|}
		\hline 
		metric & $G1$ & $G1_1$ & $G1_2$ & $G1_3$ & $G1_4$  & $G2$ & $G2_1$ & $G2_2$ & $G2_3$ & $G2_4$\\ 
		\hline \hline
		$|N|$ & 12383 &12381&12381&12381&12381&12650&12642&12642&12642&12642 \\ 
		\hline 
		$|E|$ & 22871 &22870&22870&22870&22870&23229&23224&23224&23224&23224\\ 
		\hline 
		avg-degree & 3.69394 &3.69437&3.69437&3.69437&3.69437&3.67257&3.6741&3.6741&3.6741&3.6741\\ 
		\hline 
		degree-assortavity 	& -0.26724 &-0.24973&-0.24996&-0.2497&-0.2498&-0.2541&-0.2358&-0.2358&-0.2356&-0.23565 \\ 
		\hline 
		clustering & 0.220792 &0.23462&0.23799&0.2326&0.2323&0.203&0.2164&0.22038&0.21947&0.2179 \\ 
		\hline 
		avg-distance & 3.74742 &2.85052&2.83003&2.86475&2.85751&3.75425&2.82747&2.85327&2.82148&2.80492\\ 
		\hline 
	\end{tabular} 
\end{table*}

\begin{table*}[htb!]
	
	\caption{Dataset: web-frwikinews, Basic graph properties of 1k graphs, overlap $\alpha=0.2$ and choice BFS-Tree (Highest Degree)}
	\label{tbl:dk_web-frwikinews-user-edits}
	\begin{tabular}{|c||>{\columncolor[gray]{0.8}}c||c|c|c|c||>{\columncolor[gray]{0.8}}c||c|c|c|c|}
		\hline 
		metric & $G1$ & $G1_1$ & $G1_2$ & $G1_3$ & $G1_4$  & $G2$ & $G2_1$ & $G2_2$ & $G2_3$ & $G2_4$\\ 
		\hline \hline
		$|N|$ & 13657 &13656&13656&13656&13656&12387&12342&12342&12342&12342 \\ 
		\hline 
		$|E|$ & 39243 &39242&39242&39242&39242&22204&22180&22180&22180&22180\\ 
		\hline 
		avg-degree & 5.74694 &5.74722&5.74722&5.74722&5.74722&3.58505&3.59423&3.59423&3.59423&3.59423\\ 
		\hline 
		degree-assortavity 	& -0.4354 &-0.4337&-0.4337&-0.4337&-0.4337&-0.3665&-0.3665&-0.3665&-0.3665&-0.3666 \\ 
		\hline 
		clustering & 0.1588 &0.6229&0.6242&0.6237&0.6245&0.2248&0.3745&0.3756&0.3735&0.373 \\ 
		\hline 
		avg-distance & 2.655 &2.4645&2.46895&2.467&2.4692&2.728&2.493&2.4922&2.4887&2.492\\ 
		\hline 
	\end{tabular} 
\end{table*}
